# Supplementary material for: Randomized reference models for temporal networks
Source: arXiv:1806.04032 source file (2022-12-15)
Supplement: Supplementary file 1 [file SM-Figures.tex]

%\begin{figure*}
%  \begin{tikzpicture}
%     \node at(-2.1,0){ \includegraphics[height=0.11\textheight]{{Constraints_hierarchy_v}.pdf} };
%    \node at(4.8,0){ \includegraphics[height=0.154\textheight]{{Constraints_hierarchy_v_l}.pdf} };
%   \node at(1,0){ \includegraphics[height=0.154\textheight]{{Constraints_hierarchy_v_it}.pdf} };
%    \node at(-2.3,1.6){(a)};
%    \node at(-.9,1.6){(b)};
%    \node at(4.,1.6){(c)};
%  \end{tikzpicture}
%  \caption{{\bf Hierarchies of the marginals and moments of a sequence of features.}
%  An arrow from a higher node to a lower one indicates that the former feature is finer than the latter. Thus, a MRRM that conserves the former feature necessarily conserves all  downstream features.
%  Conversely, a MRRM that randomizes a given feature also randomizes any features upstream of it as well.
%  (a) For one-level sequences of features, namely the aggregated features $\kstat$, $\a$, $\n$, $\s$, and $\w$, and $\Ebf$, and the link-timeline features $\t^1$, and $\t^w$.
%  (b) For two-level sequences of features of nodes , namely $\alphaf$, $\Dalphaf$ and $\d$. 
%  (c) For two-level sequences of features of link timelines, namely $\tauf$ and $\Dtauf$. 
%  }
%  \label{fig:constraint_hierarchy}
%\end{figure*}
%
%\begin{figure*}
%  \includegraphics[width=0.75\textwidth]{Dependency_diagram_color.pdf}
%  \caption{{\bf Feature hierarchy diagram.}
%    An arrow from a higher ranking (more central) to a lower ranking feature (vertex in the diagram) indicates that the former feature is finer than the latter. Thus, a MRRM that constrains a given feature also constrains all downstream features.
%    Conversely, a MRRM that randomizes (i.e.\ does not constrain) a given feature  does not constrain any of the upstream features either.
%    See Tables~\ref{tab:features} and \ref{tab:constraint_levels} for definitions of the features.
%   A star ($*$) emanating from a node indicates that lower hierarchical levels follow as shown in Fig.~\ref{fig:constraint_hierarchy}.
%    The color coding shows a division of features into different types: time-aggregated features (i.e.\ topological and weighted), link-timeline features, node-timeline features, and structure-aggregated features (i.e.\ purely temporal).}
%  \label{fig:dependency_diagram}
%\end{figure*}
